# Supplementary material for: Combining chains of Bayesian models with Markov melding
Source: arXiv:2111.11566 source file (2022-05-30)
Supplement: Supplementary file 1 [file 0010-stage-one-diagnostics.tex]

\begin{table}[!h]
\centering
\begin{tabular}{>{\raggedright\arraybackslash}p{2cm}rrrr}
\toprule
Parameter & $N_{\text{eff}}$ & $\widehat{R}$ & Bulk ESS & Tail ESS\\
\midrule
\cellcolor{gray!6}{$\alpha_{0}$} & \cellcolor{gray!6}{5812} & \cellcolor{gray!6}{1} & \cellcolor{gray!6}{5815} & \cellcolor{gray!6}{12113}\\
$\alpha_{2}$ & 6711 & 1 & 6722 & 14287\\
\cellcolor{gray!6}{$\rho$} & \cellcolor{gray!6}{4737} & \cellcolor{gray!6}{1} & \cellcolor{gray!6}{4767} & \cellcolor{gray!6}{4389}\\
\bottomrule
\end{tabular}
\end{table}
