# Supplementary material for: Combining chains of Bayesian models with Markov melding
Source: arXiv:2111.11566 source file (2022-05-30)
Supplement: Supplementary file 2 [file 0020-stage-two-diagnostics.tex]

\begin{table}[!h]
\centering
\begin{tabular}{>{\raggedright\arraybackslash}p{2cm}rrrr}
\toprule
Parameter & $N_{\text{eff}}$ & $\widehat{R}$ & Bulk ESS & Tail ESS\\
\midrule
\cellcolor{gray!6}{$\rho$} & \cellcolor{gray!6}{40638} & \cellcolor{gray!6}{1} & \cellcolor{gray!6}{40771} & \cellcolor{gray!6}{42893}\\
$\alpha_{0}$ & 3794 & 1 & 3708 & 2982\\
\cellcolor{gray!6}{$\alpha_{2}$} & \cellcolor{gray!6}{3071} & \cellcolor{gray!6}{1} & \cellcolor{gray!6}{3228} & \cellcolor{gray!6}{2234}\\
$\alpha_{5}$ & 1700 & 1 & 1758 & 3082\\
\bottomrule
\end{tabular}
\end{table}
