# Supplementary material for: Combining chains of Bayesian models with Markov melding
Source: arXiv:2111.11566 source file (2022-05-30)
Supplement: Supplementary file 3 [file 0021-stage-two-normal-approx-diagnostics.tex]

\begin{longtable}[t]{lrrrrrr}
\caption{\label{tab:owls-stage-two-normal-approx-diag}Numerical diagnostics for the normal approximation $\widehat{\pd}_{\text{meld}}$}\\
\toprule
  & Mean & $q_{0.05}$ & $q_{0.95}$ & $\widehat{R}$ & $\widehat{\text{ESS}}_{B}$ & $\widehat{\text{ESS}}_{T}$\\
\midrule
\endfirsthead
\caption[]{Numerical diagnostics for the normal approximation $\widehat{\pd}_{\text{meld}}$ \textit{(continued)}}\\
\toprule
  & Mean & $q_{0.05}$ & $q_{0.95}$ & $\widehat{R}$ & $\widehat{\text{ESS}}_{B}$ & $\widehat{\text{ESS}}_{T}$\\
\midrule
\endhead

\endfoot
\bottomrule
\endlastfoot
\cellcolor{gray!6}{$\rho$} & \cellcolor{gray!6}{2.31} & \cellcolor{gray!6}{2.16} & \cellcolor{gray!6}{2.46} & \cellcolor{gray!6}{1} & \cellcolor{gray!6}{7551} & \cellcolor{gray!6}{12134}\\
$\alpha_{0}$ & -2.72 & -3.12 & -2.32 & 1 & 4556 & 8011\\
\cellcolor{gray!6}{$\alpha_{2}$} & \cellcolor{gray!6}{2.43} & \cellcolor{gray!6}{1.98} & \cellcolor{gray!6}{2.90} & \cellcolor{gray!6}{1} & \cellcolor{gray!6}{4510} & \cellcolor{gray!6}{8216}\\
$\alpha_{6}$ & -0.68 & -0.94 & -0.45 & 1 & 4901 & 9199\\*
\end{longtable}
