# Supplementary material for: Combining chains of Bayesian models with Markov melding
Source: arXiv:2111.11566 source file (2022-05-30)
Supplement: Supplementary file 4 [file 0022-stage-two-lin-pooling-diagnostics.tex]

\begin{longtable}[t]{lrrrrrr}
\caption{\label{tab:owls-stage-two-log-diag}Numerical diagnostics for the melded posterior using linear pooling $\pd_{\text{meld, log}}$}\\
\toprule
  & Mean & $q_{0.05}$ & $q_{0.95}$ & $\widehat{R}$ & $\widehat{\text{ESS}}_{B}$ & $\widehat{\text{ESS}}_{T}$\\
\midrule
\endfirsthead
\caption[]{Numerical diagnostics for the melded posterior using linear pooling $\pd_{\text{meld, log}}$ \textit{(continued)}}\\
\toprule
  & Mean & $q_{0.05}$ & $q_{0.95}$ & $\widehat{R}$ & $\widehat{\text{ESS}}_{B}$ & $\widehat{\text{ESS}}_{T}$\\
\midrule
\endhead

\endfoot
\bottomrule
\endlastfoot
\cellcolor{gray!6}{$\alpha_{0}$} & \cellcolor{gray!6}{-2.76} & \cellcolor{gray!6}{-3.16} & \cellcolor{gray!6}{-2.37} & \cellcolor{gray!6}{1} & \cellcolor{gray!6}{58168} & \cellcolor{gray!6}{38197}\\
$\alpha_{2}$ & 2.45 & 2.00 & 2.92 & 1 & 57127 & 37315\\
\cellcolor{gray!6}{$\rho$} & \cellcolor{gray!6}{2.31} & \cellcolor{gray!6}{2.17} & \cellcolor{gray!6}{2.46} & \cellcolor{gray!6}{1} & \cellcolor{gray!6}{78003} & \cellcolor{gray!6}{76998}\\*
\end{longtable}
