# Supplementary material for: Combining chains of Bayesian models with Markov melding
Source: arXiv:2111.11566 source file (2022-05-30)
Supplement: Supplementary file 7 [file 0011-orig-ipm-diagnostics.tex]

\begin{longtable}[t]{lrrrrrr}
\caption{\label{tab:owls-orig-ipm-diag}Numerical diagnostics for the original IPM.}\\
\toprule
  & Mean & $q_{0.05}$ & $q_{0.95}$ & $\widehat{R}$ & $\widehat{\text{ESS}}_{B}$ & $\widehat{\text{ESS}}_{T}$\\
\midrule
\endfirsthead
\caption[]{Numerical diagnostics for the original IPM. \textit{(continued)}}\\
\toprule
  & Mean & $q_{0.05}$ & $q_{0.95}$ & $\widehat{R}$ & $\widehat{\text{ESS}}_{B}$ & $\widehat{\text{ESS}}_{T}$\\
\midrule
\endhead

\endfoot
\bottomrule
\endlastfoot
\cellcolor{gray!6}{$\alpha_{0}$} & \cellcolor{gray!6}{-2.72} & \cellcolor{gray!6}{-3.12} & \cellcolor{gray!6}{-2.34} & \cellcolor{gray!6}{1} & \cellcolor{gray!6}{4282} & \cellcolor{gray!6}{10106}\\
$\alpha_{1}$ & 2.43 & 1.98 & 2.89 & 1 & 4591 & 9960\\
\cellcolor{gray!6}{$\alpha_{2}$} & \cellcolor{gray!6}{-0.04} & \cellcolor{gray!6}{-0.45} & \cellcolor{gray!6}{0.36} & \cellcolor{gray!6}{1} & \cellcolor{gray!6}{12748} & \cellcolor{gray!6}{31064}\\
$\alpha_{4}$ & -0.01 & -3.31 & 3.28 & 1 & 120346 & 120006\\
\cellcolor{gray!6}{$\alpha_{5}$} & \cellcolor{gray!6}{-1.16} & \cellcolor{gray!6}{-1.83} & \cellcolor{gray!6}{-0.51} & \cellcolor{gray!6}{1} & \cellcolor{gray!6}{30268} & \cellcolor{gray!6}{46741}\\
$\alpha_{6}$ & -0.68 & -0.93 & -0.45 & 1 & 8534 & 15658\\
\cellcolor{gray!6}{$\rho$} & \cellcolor{gray!6}{2.31} & \cellcolor{gray!6}{2.16} & \cellcolor{gray!6}{2.46} & \cellcolor{gray!6}{1} & \cellcolor{gray!6}{66384} & \cellcolor{gray!6}{67601}\\
$\alpha_{5, 1}$ & -0.51 & -1.97 & 0.87 & 1 & 68633 & 62766\\
\cellcolor{gray!6}{$\alpha_{5, 2}$} & \cellcolor{gray!6}{1.33} & \cellcolor{gray!6}{0.24} & \cellcolor{gray!6}{2.51} & \cellcolor{gray!6}{1} & \cellcolor{gray!6}{62022} & \cellcolor{gray!6}{62242}\\
$\alpha_{5, 3}$ & 1.09 & -0.07 & 2.31 & 1 & 60480 & 63642\\
\cellcolor{gray!6}{$\alpha_{5, 4}$} & \cellcolor{gray!6}{1.98} & \cellcolor{gray!6}{0.81} & \cellcolor{gray!6}{3.28} & \cellcolor{gray!6}{1} & \cellcolor{gray!6}{57053} & \cellcolor{gray!6}{58788}\\
$\alpha_{5, 5}$ & 0.51 & -0.76 & 1.80 & 1 & 63365 & 65790\\
\cellcolor{gray!6}{$\alpha_{5, 6}$} & \cellcolor{gray!6}{-2.52} & \cellcolor{gray!6}{-4.71} & \cellcolor{gray!6}{-0.69} & \cellcolor{gray!6}{1} & \cellcolor{gray!6}{69656} & \cellcolor{gray!6}{61501}\\
$\alpha_{5, 7}$ & 1.63 & 0.34 & 3.02 & 1 & 55180 & 60856\\
\cellcolor{gray!6}{$\alpha_{5, 8}$} & \cellcolor{gray!6}{1.08} & \cellcolor{gray!6}{-0.17} & \cellcolor{gray!6}{2.38} & \cellcolor{gray!6}{1} & \cellcolor{gray!6}{54242} & \cellcolor{gray!6}{61416}\\
$\alpha_{5, 9}$ & 0.53 & -1.16 & 2.19 & 1 & 61599 & 65485\\
\cellcolor{gray!6}{$\alpha_{5, 10}$} & \cellcolor{gray!6}{1.85} & \cellcolor{gray!6}{-0.36} & \cellcolor{gray!6}{4.27} & \cellcolor{gray!6}{1} & \cellcolor{gray!6}{69799} & \cellcolor{gray!6}{65187}\\
$\alpha_{5, 11}$ & -0.48 & -2.39 & 1.32 & 1 & 69734 & 62810\\
\cellcolor{gray!6}{$\alpha_{5, 12}$} & \cellcolor{gray!6}{1.70} & \cellcolor{gray!6}{0.22} & \cellcolor{gray!6}{3.36} & \cellcolor{gray!6}{1} & \cellcolor{gray!6}{68203} & \cellcolor{gray!6}{63589}\\
$\alpha_{5, 13}$ & 0.59 & -0.87 & 2.09 & 1 & 65984 & 65000\\
\cellcolor{gray!6}{$\alpha_{5, 14}$} & \cellcolor{gray!6}{0.84} & \cellcolor{gray!6}{-0.51} & \cellcolor{gray!6}{2.28} & \cellcolor{gray!6}{1} & \cellcolor{gray!6}{68050} & \cellcolor{gray!6}{64442}\\
$\alpha_{5, 15}$ & -2.17 & -4.46 & -0.20 & 1 & 70475 & 63755\\
\cellcolor{gray!6}{$\alpha_{5, 16}$} & \cellcolor{gray!6}{2.45} & \cellcolor{gray!6}{0.53} & \cellcolor{gray!6}{4.68} & \cellcolor{gray!6}{1} & \cellcolor{gray!6}{68163} & \cellcolor{gray!6}{59726}\\
$\alpha_{5, 17}$ & -2.26 & -4.51 & -0.35 & 1 & 70746 & 61183\\
\cellcolor{gray!6}{$\alpha_{5, 18}$} & \cellcolor{gray!6}{-0.41} & \cellcolor{gray!6}{-1.85} & \cellcolor{gray!6}{0.95} & \cellcolor{gray!6}{1} & \cellcolor{gray!6}{70111} & \cellcolor{gray!6}{65283}\\
$\alpha_{5, 19}$ & -2.30 & -4.57 & -0.39 & 1 & 71720 & 61270\\
\cellcolor{gray!6}{$\alpha_{5, 20}$} & \cellcolor{gray!6}{0.26} & \cellcolor{gray!6}{-1.09} & \cellcolor{gray!6}{1.60} & \cellcolor{gray!6}{1} & \cellcolor{gray!6}{71284} & \cellcolor{gray!6}{69952}\\
$\alpha_{5, 21}$ & 0.60 & -0.68 & 1.90 & 1 & 64884 & 63487\\
\cellcolor{gray!6}{$\alpha_{5, 22}$} & \cellcolor{gray!6}{1.68} & \cellcolor{gray!6}{0.27} & \cellcolor{gray!6}{3.27} & \cellcolor{gray!6}{1} & \cellcolor{gray!6}{64016} & \cellcolor{gray!6}{59300}\\
$\alpha_{5, 23}$ & -0.67 & -2.10 & 0.70 & 1 & 69500 & 66089\\
\cellcolor{gray!6}{$\alpha_{5, 24}$} & \cellcolor{gray!6}{0.05} & \cellcolor{gray!6}{-1.36} & \cellcolor{gray!6}{1.52} & \cellcolor{gray!6}{1} & \cellcolor{gray!6}{59708} & \cellcolor{gray!6}{62276}\\
$\alpha_{5, 25}$ & 1.56 & -0.26 & 3.88 & 1 & 49486 & 54344\\*
\end{longtable}
